# Supplementary material for: The Scientific Evidence Indicator for Popular Science News
Source: arXiv:2201.03363 source file (2022-01-10)
Supplement: Supplementary file 1 [file appendix.tex]

\section{Visual vocabulary of an Elementary System Net}
\label{app:elsysnet}

\begin{figure}
    \includegraphics[scale=1]{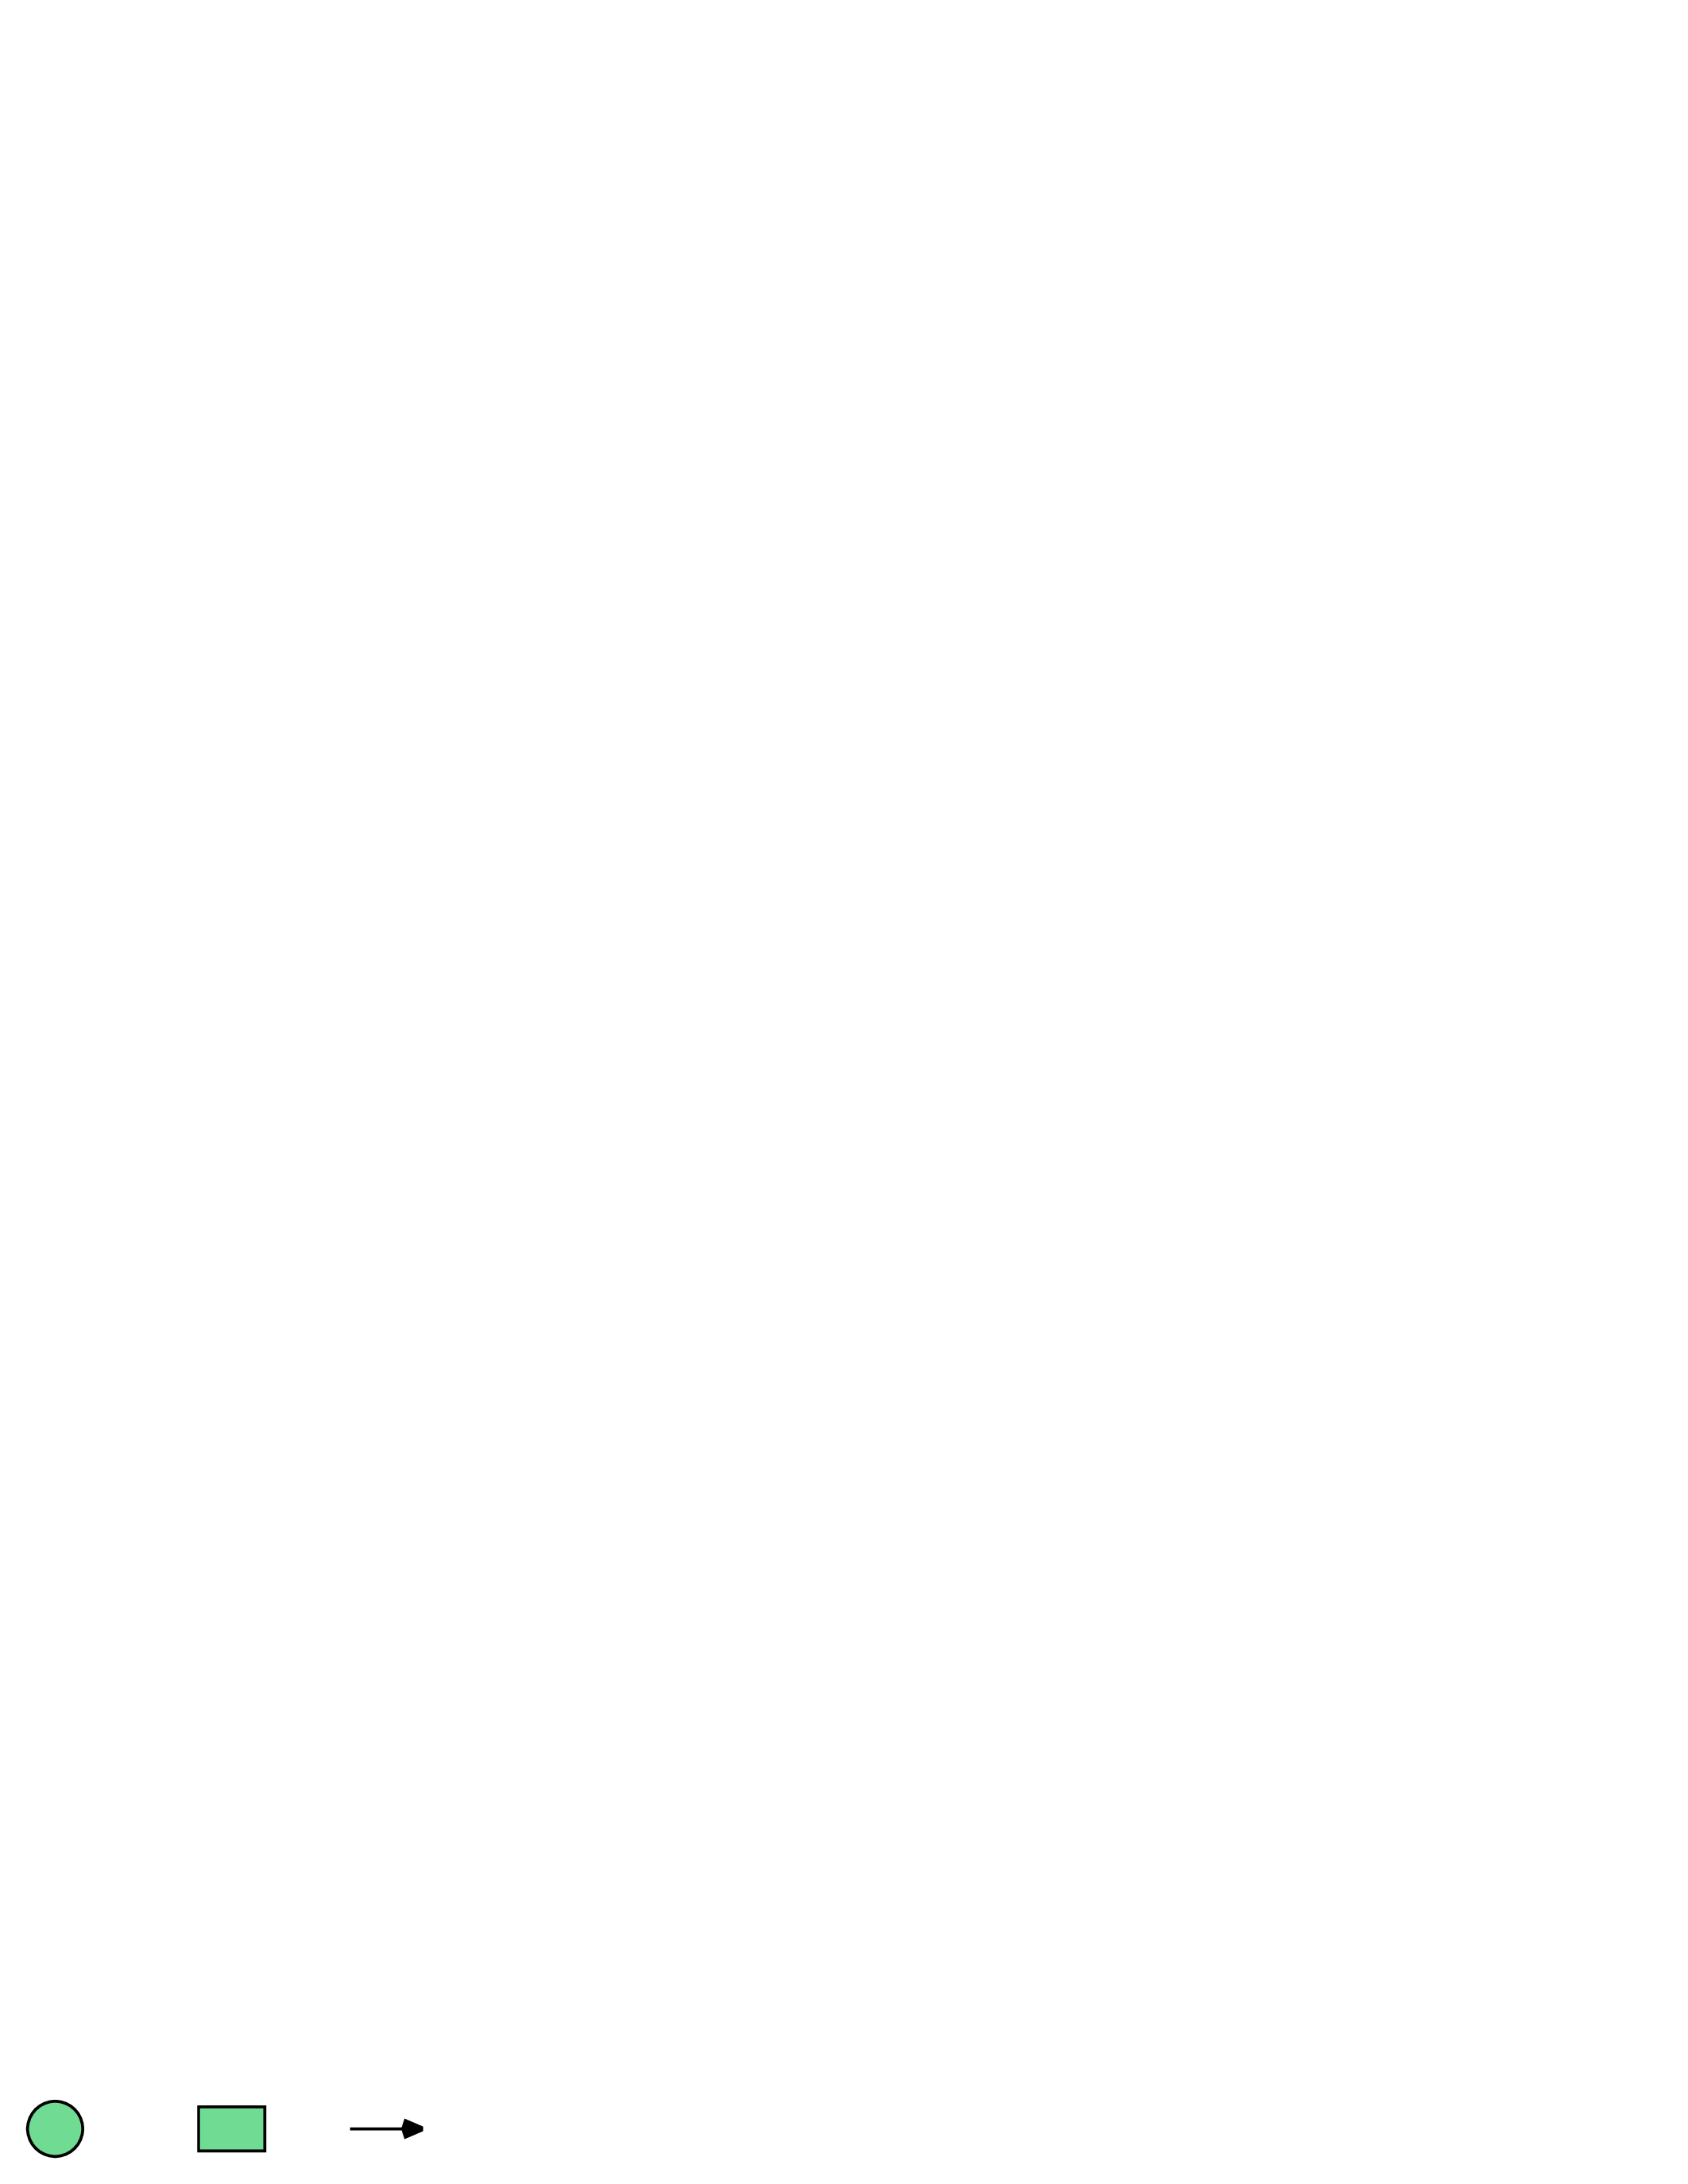}
    \caption{A circle depicts a place, a rectangle depicts a transition and an arrow depicts and arc. The arrow connects places with transitions and can be bent for that purpose. The green color is the standard color of the }
    \label{fig:visual_vocabulary_elementary_system_net}
\end{figure}
